# Supplementary material for: CADENet: Condition-Adaptive Asynchronous Dual-Stream Enhancement Network for Adverse Weather Perception in Autonomous Driving
Source: arXiv:2605.19837 source file (2026-05-19)
Supplement: Supplementary file 1 [file Appendix.tex]

% ---------------------------------------------------------------
% Appendix.tex — Ablation and supplementary material
% ---------------------------------------------------------------
\appendix
\section{Ablation Study Design}
\label{sec:ablation}

The following ablation studies are designed to isolate each
CADENet component's contribution.
Results on the full 1,327-image DAWN set are reserved for the
extended version; Table~\ref{tab:ablation} lists the planned
configurations.

\begin{table}[h]
\centering
\caption{Planned ablation configurations.}
\label{tab:ablation}

\setlength{\tabcolsep}{3pt}
\begin{tabular}{cll}
\toprule
ID & Modification & Expected Effect \\
\midrule
A1 & Async $\to$ blocking single-thread & Thread~S FPS collapses \\
A2 & PEE $\to$ uniform $R(j)=0.5$ & Rain patch discrimination lost \\
A3 & Severity $\to$ fixed $s=0.6$ & CAPE less adaptive \\
A4 & CAPE $\to$ pass-through & $F_1$ converges to C1 baseline \\
A5 & EG-NMS $\to$ Thread~S only & Removes quality refinement \\
A6 & KTT $\to$ raw detections & Temporal jitter \\
A7 & Thread~E disabled & Thread~Q latency $+50$\,ms CPU \\
\bottomrule
\end{tabular}
\end{table}

A1 directly demonstrates the production cost of blocking enhancement:
Thread~S FPS drops from $>\!60$ to $\sim\!9$--12\,FPS.
A2 shows PEE's contribution to rain handling specifically.
A7 demonstrates Thread~E's latency benefit: without it, ResNet50
embedding runs sequentially in Thread~Q, increasing Thread~Q
latency by ${\sim}50$\,ms CPU and delaying the SED recommendation
past CAPE's decision point, providing zero pre-CAPE guidance.

\section{Filter Configuration Details}

The default CAPE parameters (Table~\ref{tab:cape_params}) are
stored in \texttt{filter\_configs/default.json} and are the
parameters used for all benchmark results in this paper.

\begin{table}[h]
\centering
\caption{Default CAPE filter parameters.}
\label{tab:cape_params}

\setlength{\tabcolsep}{4pt}
\begin{tabular}{llll}
\toprule
Condition & Parameter & Value & Note \\
\midrule
\multirow{5}{*}{Rain}
  & \texttt{inpaint\_method} & TELEA & \cite{telea2004inpaint} \\
  & \texttt{inpaint\_radius} & 3 & pixels \\
  & \texttt{clahe\_clip} & 1.5 & Stage~4 \\
  & \texttt{bilateral\_d} & 5 & Stage~5 \\
  & \texttt{bilateral\_$\sigma$} & 40 & Stage~5 \\
\midrule
\multirow{3}{*}{Fog}
  & \texttt{method} & DCP & \cite{he2011dcp} \\
  & \texttt{dcp\_kernel} & 15 & patch size \\
  & \texttt{atm\_pct} & 0.001 & top-0.1\% \\
\midrule
Sand & \texttt{clahe\_clip} & 2.0 & \\
Snow & \texttt{clahe\_clip} & 2.0 & \\
\bottomrule
\end{tabular}
\end{table}
